# Supplementary material for: Susceptibility of Polar Flocks to Spatial Anisotropy
Source: arXiv:2201.00704 ancillary file (2022-01-04)
Supplement: Supplementary file 1 [file Supp_v3.pdf]

# Supplementary Information for: "Susceptibility of Polar Flocks to Spatial Anisotropy"

Alexandre Solon,[1] Hugues Chaté,[2,3,1] John Toner,[4] and Julien Tailleur[5]

[1] *Sorbonne Université, CNRS, Laboratoire de Physique Théorique de la Matière Condensée, 75005 Paris, France*

[2] *Service de Physique de l'Etat Condensé, CEA, CNRS Université Paris-Saclay, CEA-Saclay, 91191 Gif-sur-Yvette, France*

[3] *Computational Science Research Center, Beijing 100094, China*

[4] *Department of Physics and Institute for Fundamental Science, University of Oregon, Eugene, OR 97403*

[5] *Université de Paris, Laboratoire Matière et Systèmes Complexes (MSC), UMR 7057 CNRS,F-75205 Paris, France*

## I. CONTINUOUS SPIN LIMIT

Let us consider, in the active $q$-state clock model, the dynamics of a given spin $i$ oriented in direction $\theta$ that is on site $\mathbf{R}$ having density and magnetization $(\rho_\mathbf{R},\, \mathbf{m}_\mathbf{R})$. Let us write $W^\pm(\theta)$ the rate to switch from $\theta$ to the next or previous hour $\theta \pm d\theta$ with $d\theta = 2\pi/q$. These rates, given in Eq. (1) of the main text, read

$$W^\pm(\theta) = w_0 \exp\left[\tfrac{\beta}{2\rho_\mathbf{R}} \mathbf{m}_\mathbf{R} \cdot (\mathbf{u}^\pm - \mathbf{u})\right] \tag{1}$$

with $\mathbf{u} = (\cos\theta, \sin\theta)$ and $\mathbf{u}^\pm = (\cos(\theta \pm d\theta), \sin(\theta \pm d\theta))$. The corresponding master equation is given by:

$$\partial_t P(\theta) = W^+(\theta - d\theta)P(\theta - d\theta) + W^-(\theta + d\theta)P(\theta + d\theta) - \left[W^+(\theta) + W^-(\theta)\right] P(\theta) \tag{2}$$

When $q \to \infty$, we can expand Eq. (2) in powers of $d\theta$. To second order, this yields a Fokker-Planck equation

$$\partial_t P(\theta) = -\frac{\partial}{\partial\theta}\left[\Omega_\infty P\right] + \frac{\partial^2}{\partial\theta^2}\left[D_\infty P\right] \tag{3}$$

with the coefficients

$$\Omega_\infty = (W^+ - W^-)d\theta = \frac{4w_0\pi^2\beta}{q^2}\left(\frac{\mathbf{m}_\mathbf{R}}{\rho_\mathbf{R}} \cdot \frac{\partial \mathbf{u}}{\partial\theta}\right) + O(q^{-3}) \tag{4}$$

$$D_\infty = \frac{(W^+ + W^-)}{2} d\theta^2 = \frac{4w_0\pi^2}{q^2} + O(q^{-3}) \tag{5}$$

To have a well-behaved $q = \infty$ limit, with non-vanishing drift and diffusion coefficients, we thus need to take $w_0 \propto q^2$. In all the paper, we use $w_0 = q^2/(4\pi^2)$ so that $D_\infty = 1$. With this choice of coefficients and to leading order in $q$, Eq. (3) for the spin $i$ can be recast as the Langevin equation

$$\dot\theta = -\frac{\beta}{\rho_\mathbf{R}} \sum_{j\in\mathbf{R}} \sin(\theta - \theta_j) + \sqrt{2}\eta \tag{6}$$

with $\eta$ a unit-variance Gaussian white noise. Consistently, this can also be rewritten using the Hamiltonian that controls the spin alignment on site $\mathbf{R}$, $H_\mathbf{R} = -m_\mathbf{R}^2/(2\rho_\mathbf{R})$, as:

$$\dot\theta = -\beta\frac{\partial H_\mathbf{R}}{\partial\theta} + \sqrt{2}\eta. \tag{7}$$

## II. MEAN-FIELD "CLOCK POTENTIAL"

We show in this section that the discretization of the angle acts as a pinning field for the global magnetization, aligning it with the $q$ hours of the clock. To do so, we use the Bragg-Williams mean-field approach, as presented *e.g.* in Ref. [? ], and compute the effective potential $V(\phi)$ acting on the angle $\phi$ of the magnetization.

We start from a fully-connected clock model (as are all the sites of our active clock model in the absence of particle jumps) with Hamiltonian $H = -m^2/(2N)$ where $\mathbf{m}$ is the magnetization and $N$ the number of particles. We also define the polarity $\mathbf{p} = \mathbf{m}/N$, whose magnitude and direction are given by $\mathbf{p} = p(\cos\phi_p, \sin\phi_p)$. The partition function reads

$$Z = \sum_\mathcal{C} \exp\left(\frac{\beta N p(\mathcal{C})^2}{2}\right) \tag{8}$$

with $\mathcal{C}$ a microscopic configuration of the $N$ spins. We rewrite Eq. (8) by grouping all the configurations having the same $\mathbf{p}$ to get

$$Z = \int d\mathbf{p} \exp\left(\frac{\beta N p^2}{2} + \frac{S(\mathbf{p})}{k_B}\right) \tag{9}$$

with the entropy $S(\mathbf{p}) = k_B \log\Omega(\mathbf{p})$ where $\Omega(\mathbf{p})$ is the number of configurations with polarity $\mathbf{p}$. We can now introduce the free energy per particle $f(\mathbf{p})$ so that Eq. (9) becomes

$$Z = \int d\mathbf{p} \exp\left(-N\beta f(\mathbf{p})\right); \quad f(\mathbf{p}) = -\frac{p^2}{2} - Ts(\mathbf{p}) \tag{10}$$

where $s(\mathbf{p}) = S(\mathbf{p})/N$. If we could compute $f(\mathbf{p})$, then an effective potential for the angle $\phi_p$ could be infered as $V(\phi_p) = Nf(\phi_p)$, using $P(\mathbf{p}) \sim e^{-\beta N f(\mathbf{p})}$. Since we lack an explicit expression of $s(\mathbf{p})$, we resort to a mean-field approximation, which we expect to become exact in the large $N$ limit for this fully connected system.

In practice, we consider a single particle of orientation $\mathbf{p}$, fluctuating in the effective field $\mathbf{h}$ created by its $N-1$ neighbors and assume that its entropy is equal to the entropy per particle $s(\mathbf{p})$ in the fully connected system. This approximation allows us to compute $s(\mathbf{p})$ and thus $f(\mathbf{p})$ in Sec. II A. From this we deduce the most probable value of the polarization and the effective potential that applies on the direction of polarity $\phi_p$ in Sec. II B.

### A. Free energy per particle

As argued above, we need to compute the entropy of a single spin fluctuating in the field $\mathbf{h}$ created by its neighbors. The partition function $Z_1$ for this particle reads

$$Z_1(\mathbf{h}) = \sum_{k=0}^{q-1} \exp(\beta \mathbf{h}\cdot\mathbf{u}_k) \tag{11}$$

where the $\mathbf{u}_k = (\cos(2\pi k/q), \sin(2\pi k/q))$ are the $q$ directions of the clock. Let us write $\mathbf{h} = h(\cos\phi_h, \sin\phi_h)$. Expanding the exponential, Eq. (11) reads

$$Z_1(\mathbf{h}) = \sum_{k=0}^{q-1}\sum_{n=0}^{\infty} \frac{(\beta h)^n}{n! 2^n}\left(e^{i(\phi_h - 2\pi k/q)} + e^{-i(\phi_h-2\pi k/q)}\right)^n \tag{12}$$

Expanding each term and summing over $k$, we can reorder Eq. (12) as the series

$$Z_1(\mathbf{h}) = qI_0(\beta h) + \sum_{\ell=1}^{\infty} 2qI_{q\ell}(\beta h)\cos(\ell q\phi_h) \tag{13}$$

where $I_n(x) = \sum_{k=0}^{\infty}\left(\frac{x}{2}\right)^{2k+n}\frac{1}{k!(k+n)!}$ is the modified Bessel function of the first kind.

Let us note $a(\mathbf{h}) = -\log Z_1/\beta$ the Gibbs free energy of the spin. We now compute the entropy of the system when the average orientation $\langle\mathbf{u}\rangle$ is equal to $\mathbf{p}$. This constrains $\mathbf{h}$ to satisfy:

$$\langle\mathbf{u}\rangle = \frac{1}{Z_1}\sum_{k=0}^{q-1}\mathbf{u}_k e^{\beta\mathbf{h}\cdot\mathbf{u}_k} = -\frac{\partial a}{\partial\mathbf{h}} = \mathbf{p}. \tag{14}$$

The entropy can then be obtained from the Gibbs free energy as

$$s(\mathbf{p}) = \frac{1}{T}\big(\langle\mathbf{u}\cdot\mathbf{h}\rangle - a(h)\big) = \frac{1}{T}\left(\mathbf{p}\cdot\mathbf{h} - a(\mathbf{h})\right), \tag{15}$$

where the field $\mathbf{h}$ satisfies (14).

All in all, the free energy per particle of our fully connected system, defined in Eq. (10), now reads

$$f(\mathbf{p}) = -\frac{p^2}{2} + \mathbf{h}\cdot\mathbf{p} + a(\mathbf{h}) \tag{16}$$

where $\mathbf{h}$ is solution of Eq. (14). Contrary to the textbook case of an Ising spin, we note that the field $\mathbf{h}$, which is the field that has to be applied to a single active clock so that its average orientation is $\mathbf{p}$, need not be aligned with $\mathbf{p}$ as will become clear bellow. This is an important point since it is at the origin of the tendency of the clock model to pin the direction of polarity along the hours of the clock.

### B. Statistics of the polarity

The free energy per particle $f(\mathbf{p})$ controls the statistics of the polarity. However, we lack an explicit expression for $f$ since its expression Eq. (16) involves the field $\mathbf{h}$, which is defined as an implicit function of $\mathbf{p}$ through Eq. (14). Here we will use an expansion at large $q$ to derive explicit expressions.

Projecting Eq. (14) along the directions parallel and orthogonal to $\mathbf{h}$ leads to

$$p\cos(\phi_p - \phi_h) = -\frac{\partial a}{\partial h};\quad p\sin(\phi_p-\phi_h) = -\frac{1}{h}\frac{\partial a}{\partial\phi_h}, \tag{17}$$

where we recall that $a = -\log Z_1/\beta$ with $Z_1$ expressed as a series in Eq. (13). At large $q$, each term of the series is much smaller than the previous one: using the series representation of the Bessel function given above, one sees that $I_{q(\ell+1)}(\beta h) < \left(\frac{\beta h}{2q\ell}\right)^q I_{q\ell}(\beta h)$. In the large $q$ limit, the coefficients in the series (13) thus decrease rapidly with $\ell$ and the harmonic $\ell$ is of order $\varepsilon^\ell$ with $\varepsilon$ a small parameter. We first show below that retaining only the first term in the series yields back the mean-field theory of the standard XY model. Going one step further will lead to the effective potential on $\phi_p$.

If we retain only the zeroth order, Eq. (17) becomes

$$p\cos(\phi_p-\phi_h) = \frac{I_1(\beta h)}{I_0(\beta h)};\quad p\sin(\phi_p-\phi_h) = 0. \tag{18}$$

where we used that $I_0' = I_1$. This gives $\phi_p = \phi_h$ so that $\mathbf{h}$ and $\mathbf{p}$ are aligned. $h$ can then be obtained by inverting $p = I_1(\beta h)/I_0(\beta h)$. Going back to the free-energy Eq. (16), we see that, to this order, it does not depend on $\phi_p$. Differentiating the free energy, one has

$$\frac{\partial f}{\partial\mathbf{p}} = -\mathbf{p} + \mathbf{h}. \tag{19}$$

The most probable value $\mathbf{p}^*$ is found when the free energy is minimal, that is when $\mathbf{p}^* = \mathbf{h}$. In turn, Eq. (18) shows that $p^* = \frac{I_1(\beta p^*)}{I_0(\beta p^*)}$. To this order, there is no dependence on the orientation and all values of $\phi_p$ are equally probable: $p^*$ does not depend on $q$. This is the behavior expected for the XY model, *i.e.* in the $q\to\infty$ limit.

To understand the effect of large but finite $q$, let us go to the next order:

$$Z_1 = qI_0(\beta h) + 2qI_q(\beta h)\cos(q\phi_h) + O(\varepsilon^2)\ , \tag{20}$$

which leads to

$$a = -\frac{1}{\beta}\log I_0(\beta h) - \frac{2I_q(\beta h)}{\beta I_0(\beta h)}\cos(q\phi_h) + O(\varepsilon^2)\ . \tag{21}$$

To this order, Eq. (17) now gives

$$p\cos(\phi_p-\phi_h) = \frac{I_1}{I_0} + 2\frac{I_q' I_0 - I_1 I_q}{I_0^2}\cos(q\phi_h) \tag{22}$$

$$p\sin(\phi_p-\phi_h) = -\frac{2qI_q}{\beta I_0 h}\sin(q\phi_h) \tag{23}$$

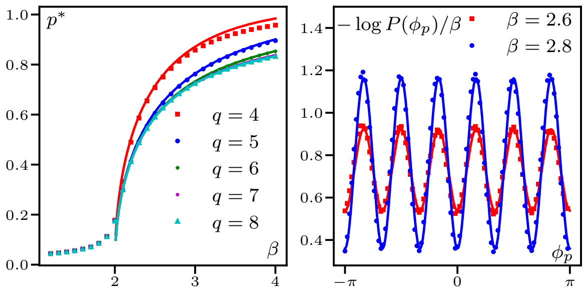


FIG. 1. Fully connected clock model (symbols) and the mean-field analytical prediction (solid lines). **Left**: average amplitude of the polarity. **Left**: Comparison on the distribution of the orientation $\phi_p$ of the order for $q = 6$. The mean-field result is expected to be exact in the limits $\rho \to \infty$ and $q \to \infty$. We use here a large $N = 1000$ and observe that the limit on $q$ is attained for relatively small values of $q$.

where all the Bessel functions are applied to $\beta h$. We see that the polarity $\mathbf{p}$ is not aligned anymore with the field $\mathbf{h}$ in general. As before, the most probable value $\mathbf{p}^*$ satisfies $\mathbf{p}^* = \mathbf{h}$ so that Eq. (22)-(23) become

$$p^* = \frac{I_1}{I_0} + 2\frac{I_q' I_0 - I_1 I_q}{I_0^2}\cos(q\phi_{p*}) \quad (24)$$

$$0 = -\frac{2qI_q}{\beta I_0 p^*}\sin(q\phi_{p*}) \quad (25)$$

where all the Bessel functions are now applied to $\beta p^*$ and we have written $\mathbf{p}^* = p^*(\cos\phi_{p*}, \sin\phi_{p*})$ in polar coordinates. Eq. (25) imposes that $\mathbf{p}^*$ be aligned with an hour of the clock, $\phi_{p*} = 2\pi k/q$ with an integer $k$ (the solutions at half hours satisfy Eq. (25) but correspond to maxima of the free energy). Eq. (24) fixes the amplitude $p^*$, and inverting it numerically, we get $p^*(\beta, q)$ which compares very well with simulations of the fully-connected model, as shown in Fig. 1 (left). Although we performed an expansion at large $q$, $p^*$ is already quite accurate for $q = 4$ and the agreement with simulations is perfect for $q > 4$.

To the same order in $\varepsilon$, we can obtain the full distribution of $\phi_p$. It comes from the free energy $f(\mathbf{p})$ after integrating out the magnitude. To this end, we use again that $\frac{\partial f}{\partial \mathbf{p}} = -\mathbf{p} + \mathbf{h}$ and project on the direction orthogonal to $\mathbf{p}$ to get

$$\frac{1}{p}\frac{\partial f}{\partial \phi_p} = h\sin(\phi_h - \phi_p) \quad (26)$$

To leading order, we use Eq. (23) to obtain

$$\frac{\partial f}{\partial \phi_p} = \frac{2qI_q(\beta p)}{\beta I_0(\beta p)}\sin(q\phi_h) = \frac{2qI_q(\beta p_0)}{\beta I_0(\beta p_0)}\sin(q\phi_p) + O(\varepsilon) \quad (27)$$

where we have replaced $\phi_h$ by $\phi_p$ in the last equality since $\phi_p - \phi_h$ is itself of order $\varepsilon$, as clear from Eq. (23). Likewise, $p$ was replaced by $p_0$ the magnetization obtained at zeroth order. Finally, we can integrate Eq. (27) with respect to $\phi_p$ to get the free energy

$$f(\phi_p) = -\frac{2I_q(\beta p_0)}{\beta I_0(\beta p_0)}\cos(q\phi_p) + K(p) \quad (28)$$

with some function $K$ that does not depend on the angle $\phi_p$. To this order, the angle of the magnetization may thus fluctuate and its statistics is given by the distribution $P(\phi_p) \propto e^{-\beta N f(\phi_p)}$. In turns, this allows identifying the effective potential $V(\phi_p) = Nf(\phi_p)$. Fig. 1 compares this result to numerical simulations. Note that our mean-field predictions are expected to become exact in the limits $N \to \infty$ and $q \to \infty$. In comparing with simulations we use a large $N = 1000$ to look at the convergence in $q$. We see that already for $q = 6$ the agreement is very good.

## III. MEAN-FIELD HYDRODYNAMIC DESCRIPTION

We derive here mean-field hydrodynamic equations for the limiting case $q \to \infty$ using standard techniques (it follows closely the derivation for the AIM [? ]).

Let us define $n_{i,j}(\theta)$ the average number of particles with orientation in $[\theta, \theta + d\theta]$ on site $(i, j)$. The hopping dynamics is the one described in the main text and the dynamics for the orientation of a spin is given by Eq. (3). The dynamics of $n_{i,j}(\theta)$ then reads

$$\begin{aligned}\dot{n}_{ij} &= D(1+\varepsilon\cos\theta)n_{i-1,j} + D(1-\varepsilon\cos\theta)n_{i+1,j} - 2Dn_{i,j} \\ &+ D(1+\varepsilon\sin\theta)n_{i,j-1} + D(1-\varepsilon\sin\theta)n_{i,j+1} - 2Dn_{i,j} \\ &- \frac{\partial}{\partial\theta}\left[\beta\frac{\mathbf{m}_{i,j}}{\rho_{i,j}}\cdot\frac{\partial\mathbf{u}(\theta)}{\partial\theta}n_{i,j}\right] + \frac{\partial^2 n_{i,j}}{\partial\theta^2} \end{aligned} \quad (29)$$

where the density and magnetization are defined as $\rho_{i,j} = \int n_{i,j}(\theta)d\theta$ and $\mathbf{m}_{i,j} = \int \mathbf{u}(\theta)n_{i,j}(\theta)d\theta$ with $\mathbf{u}(\theta) = (\cos\theta, \sin\theta)$. Note that the alignment term (*i.e.* the last line) in Eq. (29) is a mean-field term since it is derived assuming that the dynamics of a spin is independent of that of $\mathbf{m}_{i,j}$.

Let us now take the continuous limit, formally by taking the limit $a \to 0$ with $a$ the lattice spacing. The first two harmonics of Eq. (29) then read

$$\dot{\rho}(\mathbf{r}) = \tilde{D}\Delta\rho - \tilde{v}\nabla\cdot\mathbf{m} \quad (30)$$

$$\dot{\mathbf{m}}(\mathbf{r}) = \tilde{D}\Delta\mathbf{m} - \frac{\tilde{v}}{2}\nabla\rho - \frac{\tilde{v}}{2}\nabla\cdot Q + (\frac{\beta}{2} - 1)\mathbf{m} - \frac{\beta}{2\rho}Q\cdot\mathbf{m} \quad (31)$$

where $\tilde{D} = Da^2$ and $\tilde{v} = 2Da\varepsilon$ (hereafter we drop the tilde). In Eq. (31), we have defined the traceless symmetric nematic tensor $Q = \int d\theta \begin{pmatrix}\cos 2\theta & \sin 2\theta \\ \sin 2\theta & -\cos 2\theta\end{pmatrix} n(\mathbf{r}, \theta)$. One indeed obtains an infinite hierarchy of equations for the harmonics of $n(\mathbf{r}, \theta)$. To close this hierarchy, we use that the nematic tensor is a fast mode which we assume

relaxes infinitely fast, so that drift and diffusion terms can be neglected. We also neglect harmonics of higher order. This gives

$$\dot{Q}(\mathbf{r}) = 0 = \frac{\beta}{\rho}\begin{pmatrix} m_x^2 - m_y^2 & 2m_x m_y \\ 2m_x m_y & m_y^2 - m_x^2 \end{pmatrix} - 4Q \tag{32}$$

which we plug into Eq. (31) to close our system of equations, yielding

$$\begin{aligned} \dot{\rho}(\mathbf{r}) &= D\Delta\rho - v\nabla\cdot\mathbf{m} \\ \dot{\mathbf{m}}(\mathbf{r}) &= D\Delta\mathbf{m} - \frac{v}{2}\nabla\rho - \frac{v}{2}\nabla\cdot Q + (\frac{\beta}{2} - 1 - \frac{\beta^2|\mathbf{m}|^2}{8\rho^2})\mathbf{m} \\ Q &= \frac{\beta}{4\rho}\begin{pmatrix} m_x^2 - m_y^2 & 2m_x m_y \\ 2m_x m_y & m_y^2 - m_x^2 \end{pmatrix}. \end{aligned} \tag{33}$$

A direct computation of $\nabla \cdot Q$ then directly leads to Eq. (4) of the main text.

In addition, one needs to add the effect of the potential $V(\phi_p)$ induced by the discretization of the microscopic spins along the $q$ possible directions. From the previous section, we expect the potential $V$ to act on $\phi = \arg\mathbf{m}$ as $\dot{\phi} = -\Gamma\frac{\partial V}{\partial \phi}$ with a mobility coefficient $\Gamma = \beta/\rho$. This coefficient is readily obtained by imposing that, for one spin, $\partial_t\theta = \frac{1}{\rho}\partial_t\phi$ and using Eq. (7). One then uses that $\dot{m}_x = \dot{m}\cos\phi - m\dot{\phi}\sin\phi$ and similarly for $m_y$ to derive the term due to $V$ that is used in the main text.
